# Supplementary material for: Abundance of $\mathbb{Z}_2$ topological order in exfoliable two-dimensional insulators
Source: arXiv:1908.08334 ancillary file (2019-08-22)
Supplement: Supplementary file 1 [file supplementary.pdf]

# Supporting Information for

# Abundance of $\mathbb{Z}_2$ topological order in exfoliable two-dimensional insulators

Antimo Marrazzo, Marco Gibertini, Davide Campi, Nicolas Mounet, and Nicola Marzari

# $AsCuLi_2$

## Info and properties

**Formula (DB ID)** $AsCuLi_2$ (ICSD 153858)

**Spacegroup** $P\bar{6}m2$ (187)

**DFT band gap [meV]** 45

**DFT inversion strength [meV]** 80

**No. atoms per unit cell** 4

**DF2-C09 Binding energy [meV/Å$^2$]** 63

**rVV10 Binding energy [meV/Å$^2$]** 62

**$G_0W_0$ inversion strength [meV]** 169

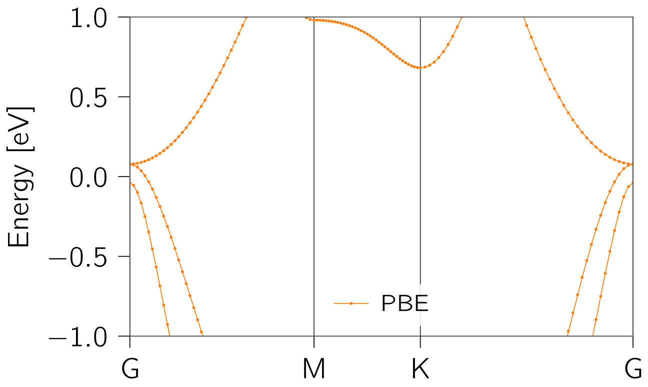


DFT band structure

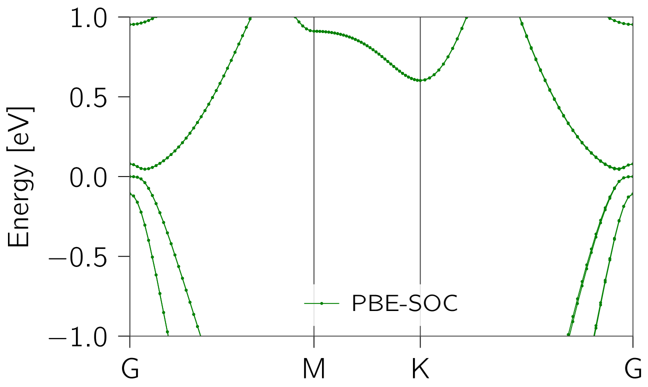


DFT band structure with spin-orbit coupling

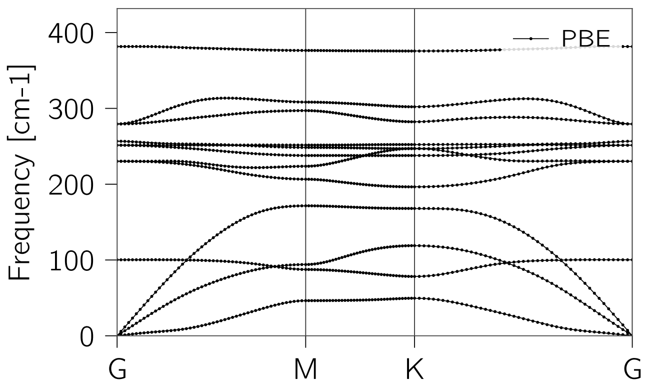


DFPT phonons dispersions

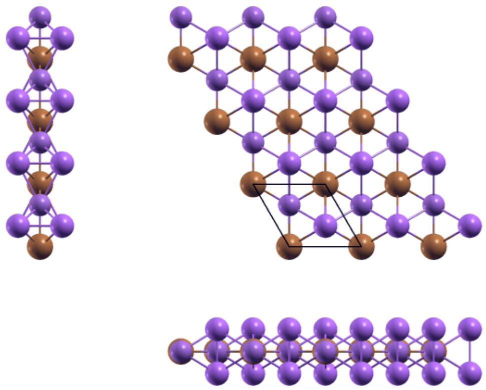

Orthographic projections Li and As atoms are purple, Cu atoms are brown.

Structural parameters: relaxed cell and atomic positions in cartesian coordinates

| | $x$ [Å] | $y$ [Å] | $z$ [Å] |
|---|---|---|---|
| $\boldsymbol{a_1}$ | 4.13516873 | −0.00000000 | 0.00000000 |
| $\boldsymbol{a_2}$ | −2.06758436 | 3.58116117 | 0.00000000 |
| $\boldsymbol{a_3}$ | 0.00000000 | 0.00000000 | 22.61983425 |
| Li | 2.06758436 | 1.19372039 | 12.57617208 |
| Li | 2.06758436 | 1.19372039 | 10.04366217 |
| Cu | −0.00000000 | 0.00000000 | 11.30991713 |
| As | 0.00000000 | 2.38744078 | 11.30991713 |

# Bi

## Info and properties

| | | | |
|---|---|---|---|
| **Formula (DB ID)** | Bi (ICSD 43938) | **No. atoms per unit cell** | 2 |
| **Spacegroup** | P$\bar{3}m1$ (164) | **DF2-C09 Binding energy [meV/Å$^2$]** | 18 |
| **DFT band gap [meV]** | 545 | **rVV10 Binding energy [meV/Å$^2$]** | 25 |
| **DFT inversion strength [meV]** | 685 | **$G_0W_0$ inversion strength [meV]** | 760 |

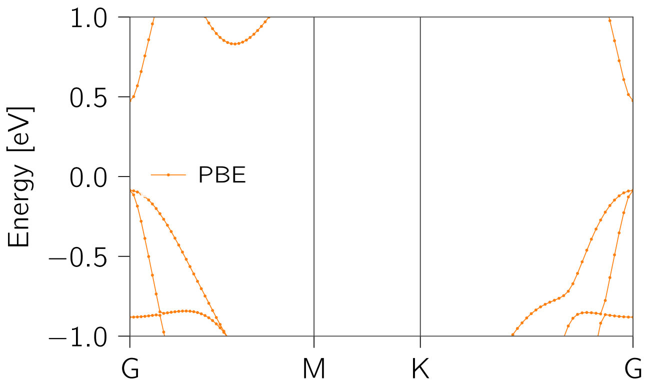


DFT band structure

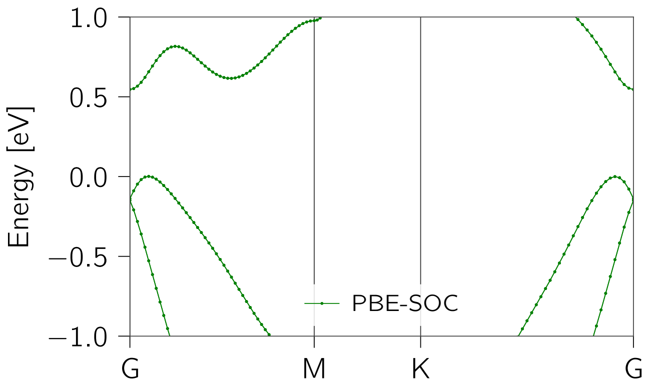


DFT band structure with spin-orbit coupling

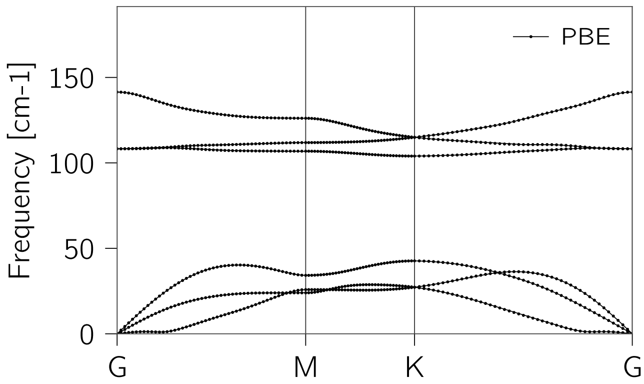


DFPT phonons dispersions

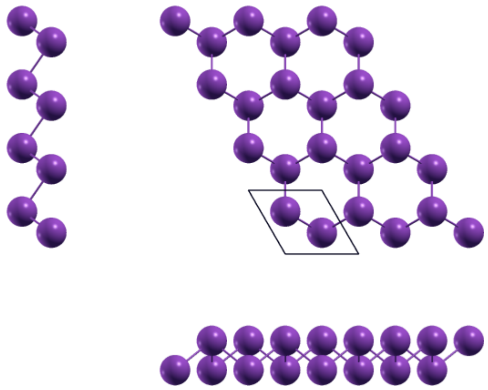

Orthographic projections

Bi atoms are purple.

Structural parameters: relaxed cell and atomic positions in cartesian coordinates

| | $x$ [Å] | $y$ [Å] | $z$ [Å] |
|---|---|---|---|
| $\boldsymbol{a_1}$ | 4.33235642 | 0.00000000 | 0.00000000 |
| $\boldsymbol{a_2}$ | −2.16617821 | 3.75193072 | 0.00000000 |
| $\boldsymbol{a_3}$ | 0.00000000 | 0.00000000 | 21.66627696 |
| ● Bi | 2.16617821 | 1.25064357 | 9.96780632 |
| ● Bi | 0.00000000 | 2.50128715 | 11.69847063 |

# ZrBr

## Info and properties

| | |
|---|---|
| **Formula (DB ID)** | ZrBr (COD 4343762) |
| **Spacegroup** | $P2_1/m$ (11) |
| **DFT band gap [meV]** | 29 (at 1 % strain) |
| **DFT inversion strength [meV]** | 45 (at 1 % strain) |

| | |
|---|---|
| **No. atoms per unit cell** | 4 |
| **DF2-C09 Binding energy [meV/Å$^2$]** | 16 |
| **rVV10 Binding energy [meV/Å$^2$]** | 22 |

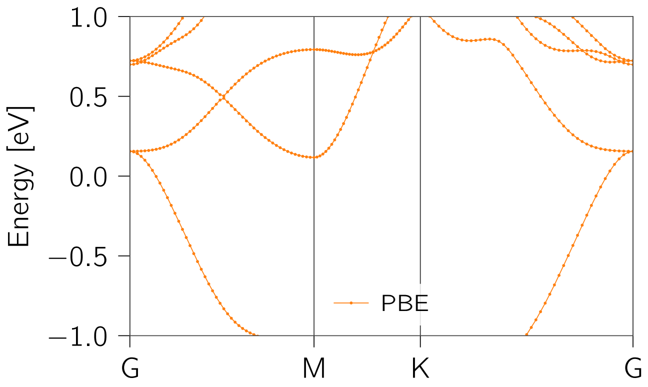


DFT band structure

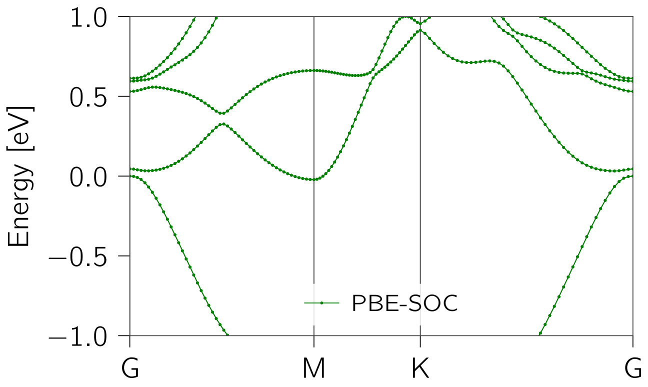


DFT band structure with spin-orbit coupling

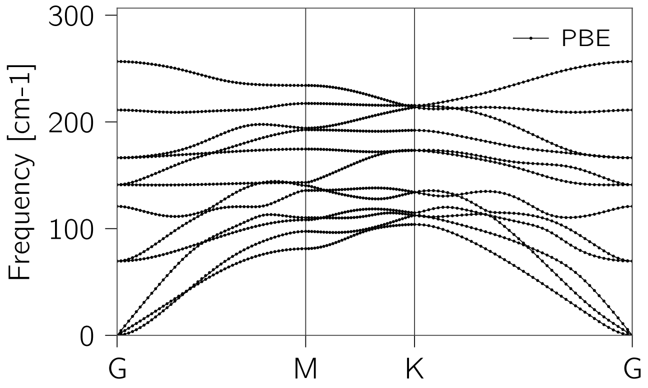


DFPT phonons dispersions

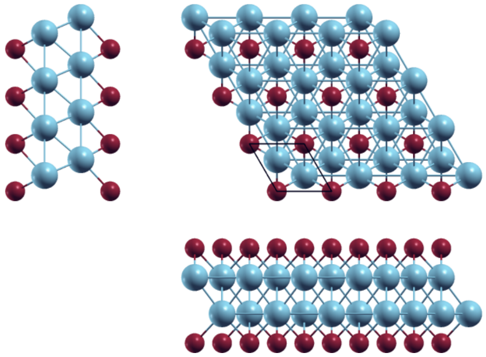

Orthographic projections

Zr atoms are light blue, Br atoms are red.

Structural parameters: relaxed cell and atomic positions in cartesian coordinates

| | $x$ [Å] | $y$ [Å] | $z$ [Å] |
|---|---|---|---|
| $\boldsymbol{a_1}$ | 3.53358354 | −0.00000000 | 0.00000000 |
| $\boldsymbol{a_2}$ | −1.76679177 | 3.06017312 | 0.00000000 |
| $\boldsymbol{a_3}$ | 0.00000000 | 0.00000000 | 26.19022272 |
| Zr | −0.00000000 | 2.04011541 | 11.92271410 |
| Br | 0.00000000 | 0.00000000 | 10.03039713 |
| Br | −0.00000000 | −0.00000000 | 16.15982559 |
| Zr | 1.76679177 | 1.02005771 | 14.26750862 |

# ZrCl

## Info and properties

**Formula (DB ID)** ZrCl (ICSD 20148)
**Spacegroup** $P2_1/m$ (11)
**DFT band gap [meV]** 39 (at 3 % strain)
**DFT inversion strength [meV]** 60 (at 3 % strain)

**No. atoms per unit cell** 4
**DF2-C09 Binding energy [meV/Å$^2$]** 15
**rVV10 Binding energy [meV/Å$^2$]** 22

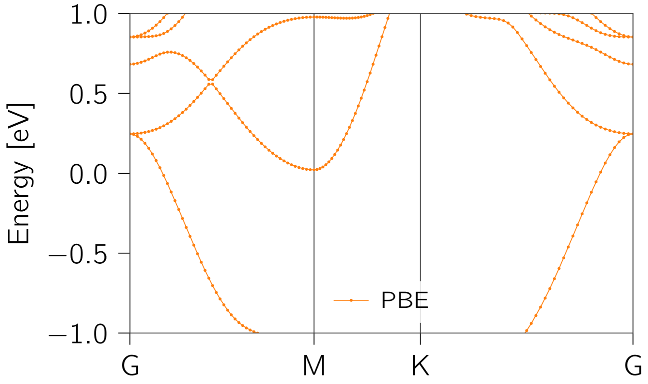


DFT band structure

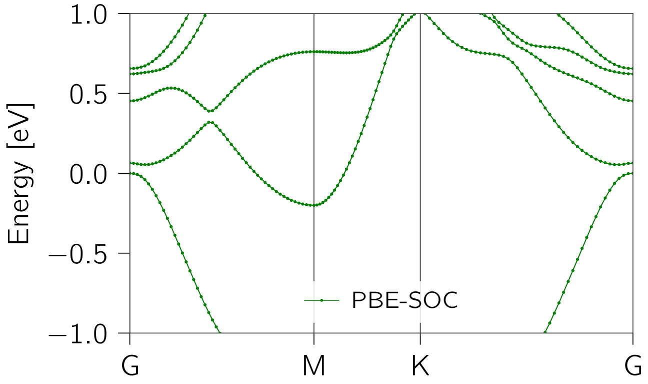


DFT band structure with spin-orbit coupling

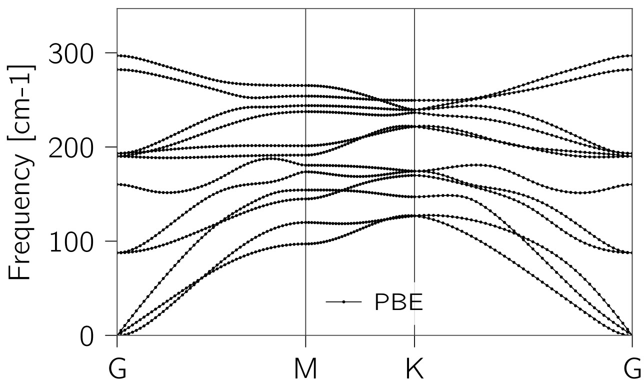


DFPT phonons dispersions

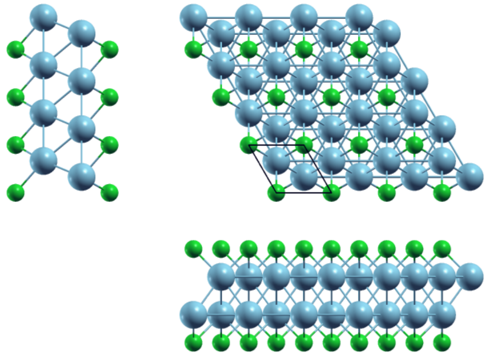

Orthographic projections
Zr atoms are light blue, Cl atoms are green.

Structural parameters: relaxed cell and atomic positions in cartesian coordinates

| | $x$ [Å] | $y$ [Å] | $z$ [Å] |
|---|---|---|---|
| $\boldsymbol{a_1}$ | 3.44582094 | 0.00000000 | 0.00000000 |
| $\boldsymbol{a_2}$ | −1.72291047 | 2.98416847 | 0.00000000 |
| $\boldsymbol{a_3}$ | 0.00000000 | 0.00000000 | 25.91026094 |
| Zr | 1.72291047 | 0.99472282 | 11.76573761 |
| Cl | 0.00000000 | −0.00000000 | 15.88438284 |
| Cl | 0.00000000 | −0.00000000 | 10.02587809 |
| Zr | 0.00000000 | 1.98944565 | 14.14452332 |

# $TiCu_2Te3$

## Info and properties

**Formula (DB ID)** $TiCu_2Te3$ (ICSD 402631)

**Spacegroup** C2/$m$ (2)

**DFT band gap [meV]** 8

**DFT inversion strength [meV]** 21

**No. atoms per unit cell** 12

**DF2-C09 Binding energy [meV/Å$^2$]** 44

**rVV10 Binding energy [meV/Å$^2$]** 44

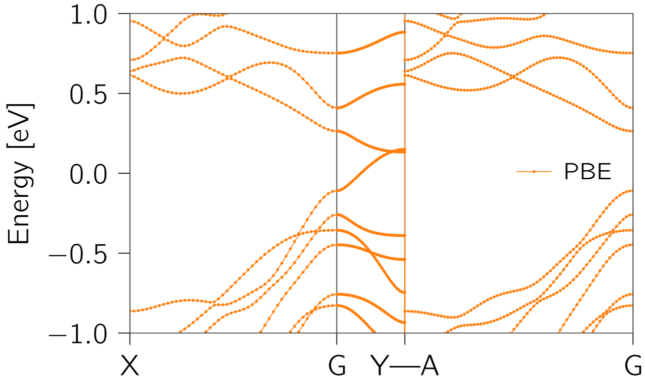


DFT band structure

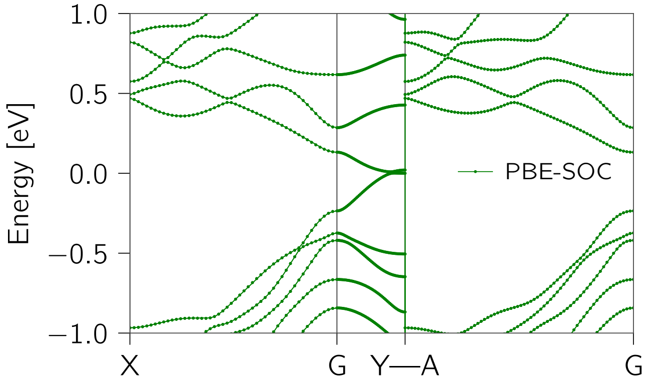


DFT band structure with spin-orbit coupling

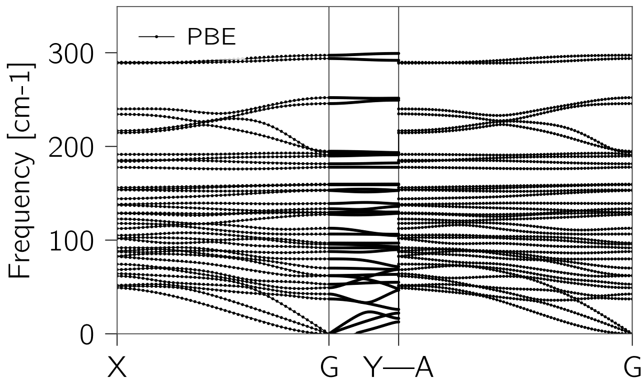


DFPT phonons dispersions

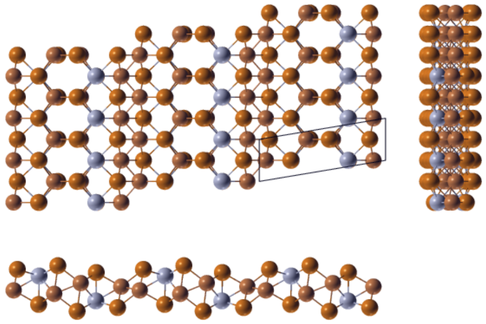

Orthographic projections

Cu and Te atoms are brown, Ti atoms are grey.

Structural parameters: relaxed cell and atomic positions in cartesian coordinates

| | $x$ [Å] | $y$ [Å] | $z$ [Å] |
|---|---|---|---|
| $\boldsymbol{a_1}$ | 3.88929588 | 0.00000062 | 0.00000000 |
| $\boldsymbol{a_2}$ | −1.94464607 | 11.65705898 | 0.00000000 |
| $\boldsymbol{a_3}$ | 0.00000000 | 0.00000000 | 24.32076299 |
| Cu | 1.94462254 | 4.86254161 | 11.66396580 |
| Te | 1.94465407 | 1.45533180 | 13.92612166 |
| Te | 1.94466036 | 5.19446772 | 14.26723669 |
| Ti | 0.00001587 | 8.71266823 | 11.00956911 |
| Ti | 0.00000892 | 3.46358329 | 13.31118999 |
| Cu | −0.00002285 | 11.06278117 | 12.33461587 |
| Cu | −0.00001264 | 1.11342181 | 11.98616866 |
| Te | 0.00001066 | 8.75426769 | 13.63462639 |
| Te | −0.00001370 | 3.42196784 | 10.68613881 |
| Cu | 1.94465306 | 7.31369238 | 12.65678717 |
| Te | 1.94465693 | 10.72092094 | 10.39463556 |
| Te | 1.94466616 | 6.98178875 | 10.05352221 |

# TiNI

## Info and properties

| | | | |
|---|---|---|---|
| **Formula (DB ID)** | TiNI (ICSD 27394) | **No. atoms per unit cell** | 6 |
| **Spacegroup** | P$mmn$(59) | **DF2-C09 Binding energy [meV/Å$^2$]** | 15 |
| **DFT band gap [meV]** | 18 | **rVV10 Binding energy [meV/Å$^2$]** | 22 |
| **DFT inversion strength [meV]** | 141 | **$G_0W_0$ inversion strength [meV]** | -705 (trivial) |

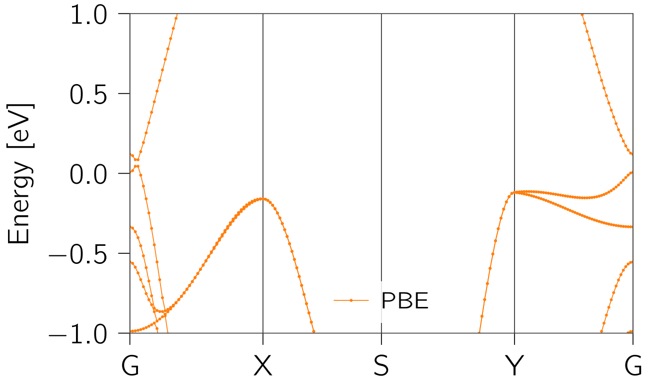


DFT band structure

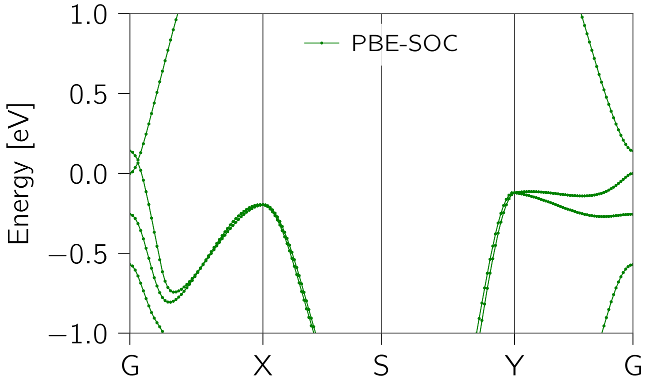


DFT band structure with spin-orbit coupling

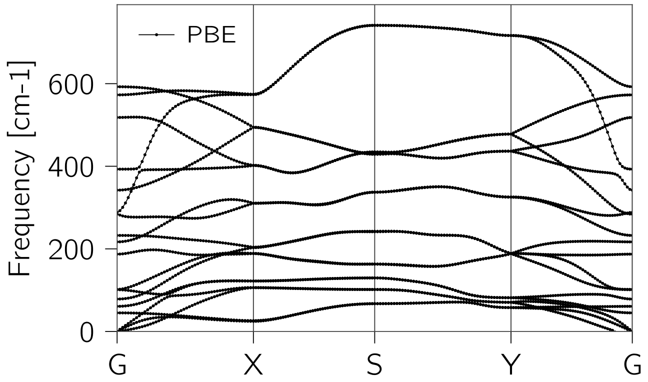


DFPT phonons dispersions

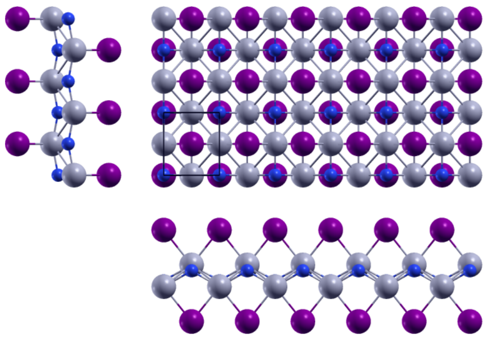

Orthographic projections

I atoms are purple, Ti atoms are grey, N atoms are blue.

Structural parameters: relaxed cell and atomic positions in cartesian coordinates

| | $x$ [Å] | $y$ [Å] | $z$ [Å] |
|---|---|---|---|
| $\boldsymbol{a_1}$ | 3.53337331 | 0.00000000 | 0.00000000 |
| $\boldsymbol{a_2}$ | 0.00000000 | 3.97007258 | 0.00000000 |
| $\boldsymbol{a_3}$ | 0.00000000 | 0.00000000 | 25.85326732 |
| Ti | 1.76668666 | 0.00000000 | 12.23631618 |
| I | 0.00000000 | 0.00000000 | 10.02286212 |
| N | 1.76668666 | 1.98503629 | 12.60851320 |
| Ti | 0.00000000 | 1.98503629 | 13.61695036 |
| I | 1.76668666 | 1.98503629 | 15.83040430 |
| N | 0.00000000 | 0.00000000 | 13.24475270 |

# $NbIrTe_4$

## Info and properties

**Formula (DB ID)** $NbIrTe_4$ (ICSD 656451)
**Spacegroup** $Pm$ (6)
**DFT band gap [meV]** 36
**DFT inversion strength [meV]** 161

**No. atoms per unit cell** 12
**DF2-C09 Binding energy [meV/Å$^2$]** 27
**rVV10 Binding energy [meV/Å$^2$]** 32

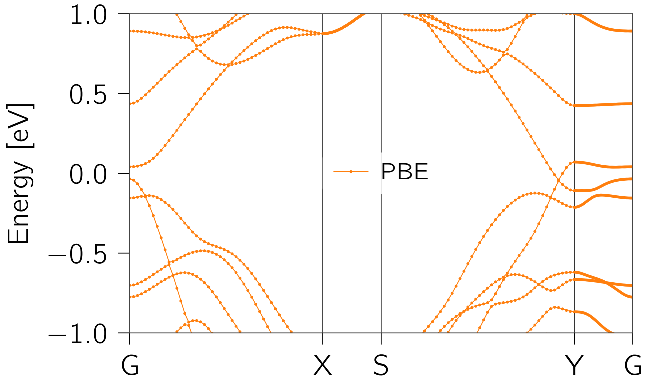


DFT band structure

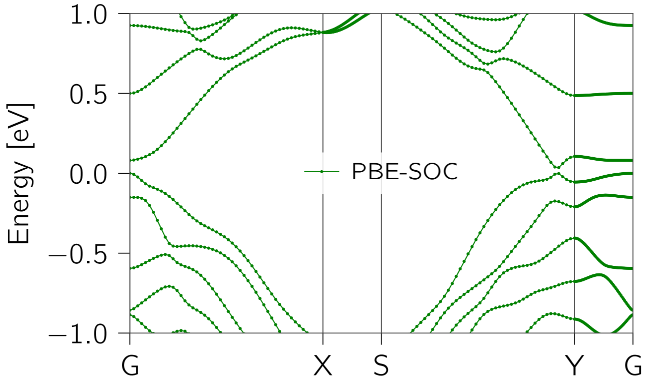


DFT band structure with spin-orbit coupling

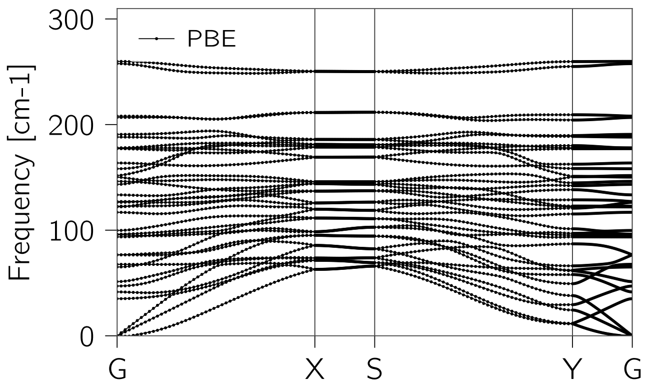


DFPT phonons dispersions

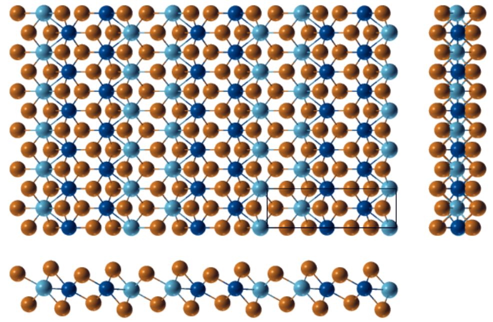

Orthographic projections
Te atoms are brown, Ir atoms are dark blue, Nb atoms are blue.

Structural parameters: relaxed cell and atomic positions in cartesian coordinates

| | $x$ [Å] | $y$ [Å] | $z$ [Å] |
|---|---|---|---|
| $\boldsymbol{a_1}$ | 3.81296741 | 0.00000000 | 0.00000000 |
| $\boldsymbol{a_2}$ | 0.00000000 | 12.60029951 | 0.00000127 |
| $\boldsymbol{a_3}$ | 0.00000000 | −0.00000238 | 38.04525154 |
| Nb | 1.90648370 | 9.20825568 | −0.09611315 |
| Te | 0.00000000 | 8.52783713 | −2.01629727 |
| Te | 1.90648370 | 5.49178472 | −1.35749642 |
| Te | 0.00000000 | 2.45131308 | −1.88684181 |
| Te | 1.90648370 | 11.77678106 | −1.49715950 |
| Ir | 1.90648370 | 3.09754442 | −0.04365771 |
| Nb | 0.00000000 | 0.65156313 | 0.09588414 |
| Te | 0.00000000 | 4.36811515 | 1.35779965 |
| Te | 0.00000000 | 10.68334976 | 1.49687553 |
| Te | 1.90648370 | 7.40888355 | 1.88696297 |
| Te | 1.90648370 | 1.33170234 | 2.01616299 |
| Ir | 0.00000000 | 6.76238094 | 0.04388058 |

# $TaIrTe_4$

## Info and properties

**Formula (DB ID)** $TaIrTe_4$ (ICSD 73322)
**Spacegroup** P$m$ (6)
**DFT band gap [meV]** 11
**DFT inversion strength [meV]** 204

**No. atoms per unit cell** 12
**DF2-C09 Binding energy [meV/Å$^2$]** 26
**rVV10 Binding energy [meV/Å$^2$]** 31

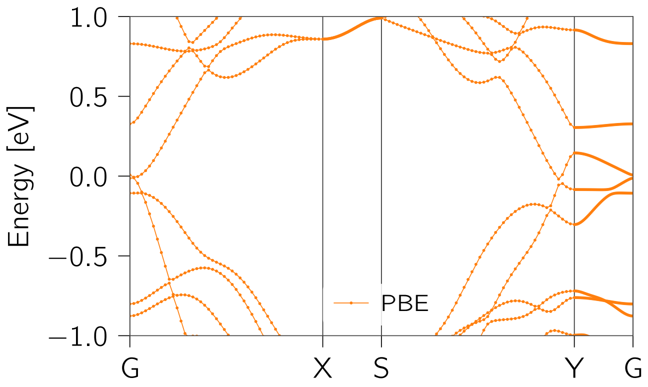


DFT band structure

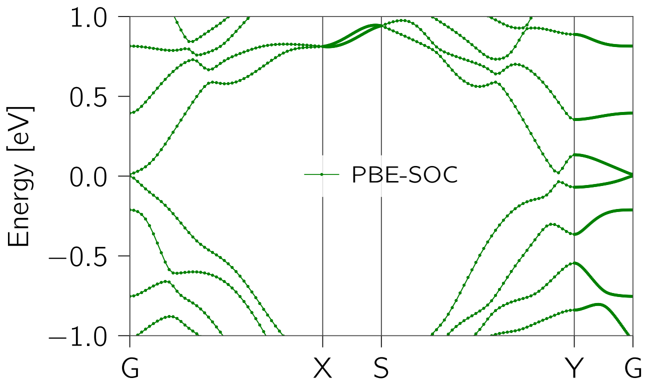


DFT band structure with spin-orbit coupling

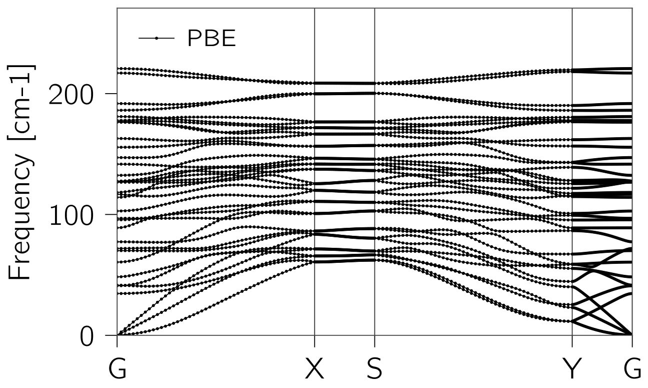


DFPT phonons dispersions

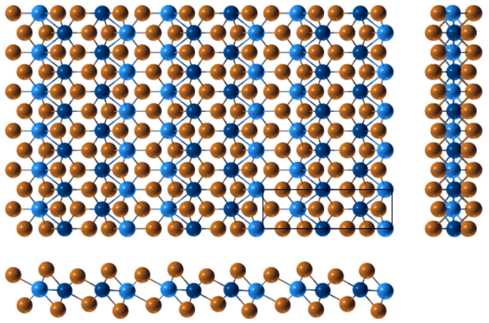

Orthographic projections

Te atoms are brown, Ir atoms are dark blue, Ta atoms are blue.

Structural parameters: relaxed cell and atomic positions in cartesian coordinates

| | $x$ [Å] | $y$ [Å] | $z$ [Å] |
|---|---|---|---|
| $\boldsymbol{a_1}$ | 3.82550686 | 0.00000000 | 0.00000000 |
| $\boldsymbol{a_2}$ | 0.00000000 | 12.57852825 | −0.00000018 |
| $\boldsymbol{a_3}$ | 0.00000000 | 0.00000035 | 24.04626477 |
| Ta | 1.91275343 | 9.18966391 | 11.91058926 |
| Te | 1.91275343 | 5.48278953 | 10.65562072 |
| Te | 0.00000000 | 2.44438928 | 10.11713155 |
| Te | 0.00000000 | 8.52896227 | 9.99161262 |
| Te | 1.91275343 | 11.76177602 | 10.53098053 |
| Ir | 1.91275343 | 3.09098423 | 11.96553811 |
| Ta | 0.00000000 | 0.65293387 | 12.10650434 |
| Te | 1.91275343 | 7.39828999 | 13.90002030 |
| Te | 1.91275343 | 1.31360315 | 14.02549820 |
| Te | 0.00000000 | 4.35981339 | 13.36152668 |
| Te | 0.00000000 | 10.65934644 | 13.48611067 |
| Ir | 0.00000000 | 6.75161872 | 12.05161112 |

# $MoTe_2$

## Info and properties

**Formula (DB ID)** $MoTe_2$ (COD 2310356)

**Spacegroup** $P2_1/m$ (11)

**DFT band gap [meV]** 26 (at 3 % strain)

**DFT inversion strength [meV]** 408

**No. atoms per unit cell** 6

**DF2-C09 Binding energy [meV/Å²]** 25

**rVV10 Binding energy [meV/Å²]** 30

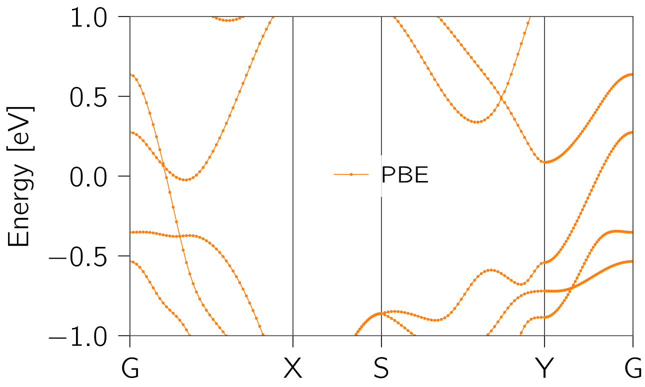


DFT band structure

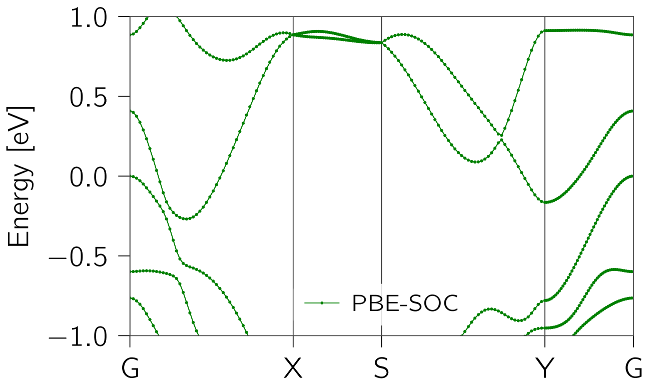


DFT band structure with spin-orbit coupling

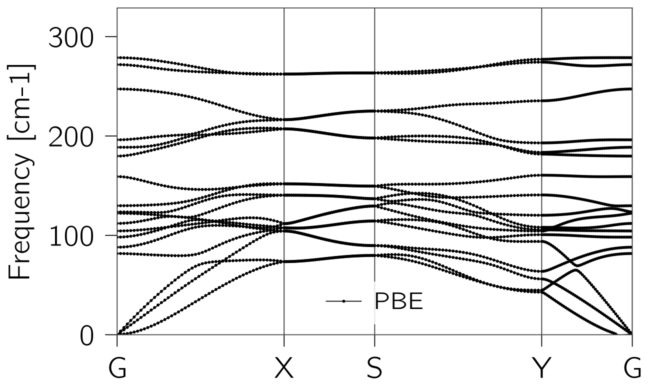


DFPT phonons dispersions

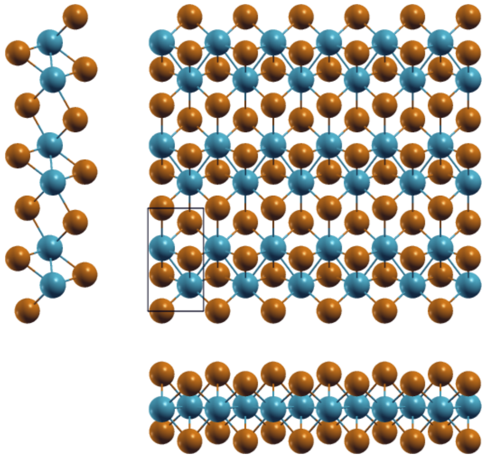

Orthographic projections

Te atoms are brown, Mo atoms are light blue.

Structural parameters: relaxed cell and atomic positions in cartesian coordinates

| | $x$ [Å] | $y$ [Å] | $z$ [Å] |
|---|---|---|---|
| $\boldsymbol{a_1}$ | 3.46007007 | 0.00000000 | 0.00000000 |
| $\boldsymbol{a_2}$ | 0.00000000 | 6.37843282 | 0.00000000 |
| $\boldsymbol{a_3}$ | 0.00000000 | 0.00000000 | 24.19479066 |
| Te | 2.59505255 | 3.26175667 | 14.17870163 |
| Te | 0.86501752 | 2.25448641 | 10.01608624 |
| Te | 0.86501752 | 0.01266770 | 13.58866831 |
| Te | 2.59505255 | 5.50356016 | 10.60612498 |
| Mo | 2.59505255 | 1.60500151 | 12.00208676 |
| Mo | 0.86501752 | 3.91118878 | 12.19270404 |

# $Pd_2HgSe_3$

## Info and properties

**Formula (DB ID)** $Pd_2HgSe_3$ (ICSD 259367)
**Spacegroup** P$\bar{3}m1$ (164)
**DFT band gap [meV]** 0
**DFT inversion strength [meV]** 80

**No. atoms per unit cell** 12
**DF2-C09 Binding energy [meV/Å$^2$]** 61
**rVV10 Binding energy [meV/Å$^2$]** 66

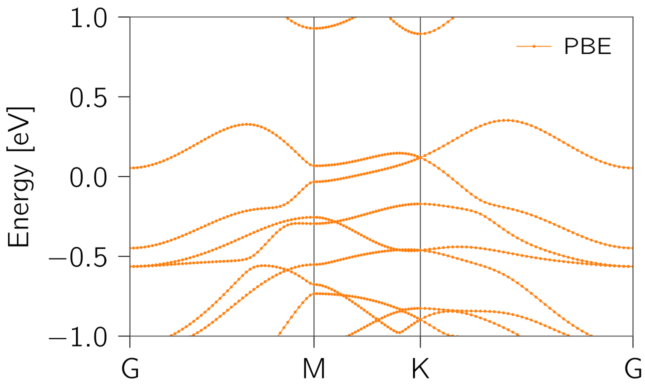


DFT band structure

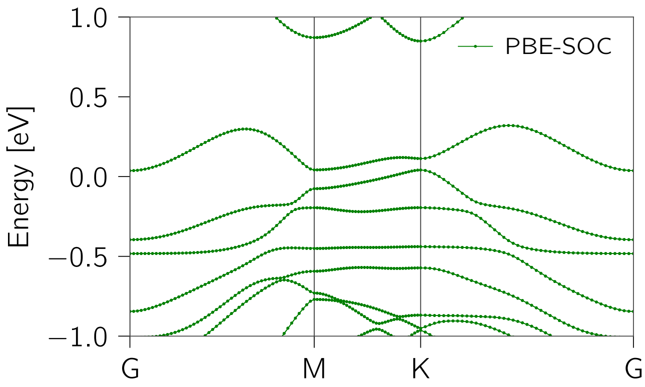


DFT band structure with spin-orbit coupling

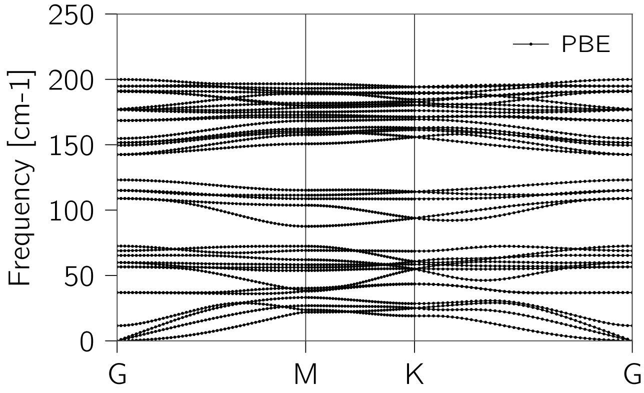


DFPT phonons dispersions

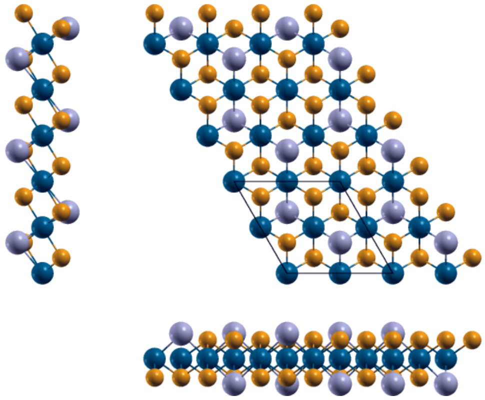

Orthographic projections

Se atoms are orange, Hg atoms are grey, Pd atoms are dark blue.

Structural parameters: relaxed cell and atomic positions in cartesian coordinates

| | $x$ [Å] | $y$ [Å] | $z$ [Å] |
|---|---|---|---|
| $\boldsymbol{a_1}$ | 7.42264912 | 0.00000000 | 0.00000000 |
| $\boldsymbol{a_2}$ | −3.71132456 | 6.42820270 | 0.00000000 |
| $\boldsymbol{a_3}$ | 0.00000000 | 0.00000000 | 27.06855346 |
| Hg | 3.71132456 | 2.14273423 | 1.76147103 |
| Hg | 0.00000000 | 4.28546847 | −1.76147103 |
| Pd | 0.00000000 | 0.00000000 | 0.00000000 |
| Pd | 5.56698684 | 3.21410135 | 0.00000000 |
| Pd | 1.85566228 | 3.21410135 | 0.00000000 |
| Pd | 3.71132456 | 0.00000000 | 0.00000000 |
| Se | 0.00000000 | 2.15447110 | 1.31323659 |
| Se | 1.84549786 | 5.35096715 | 1.31323659 |
| Se | −1.84549786 | 5.35096715 | 1.31323659 |
| Se | 3.71132456 | 4.27373160 | −1.31323659 |
| Se | 1.86582670 | 1.07723555 | −1.31323659 |
| Se | 5.55682242 | 1.07723555 | −1.31323659 |

# $Pt_2HgSe_3$

## Info and properties

| | | | |
|---|---|---|---|
| **Formula (DB ID)** | $Pt_2HgSe_3$ (ICSD 185808) | **No. atoms per unit cell** | 12 |
| **Spacegroup** | $P\bar{3}m1$ (164) | **DF2-C09 Binding energy [meV/Å$^2$]** | 60 |
| **DFT band gap [meV]** | 149 | **rVV10 Binding energy [meV/Å$^2$]** | 63 |
| **DFT inversion strength [meV]** | 168 | **$G_0W_0$ inversion strength [meV]** | 530 |

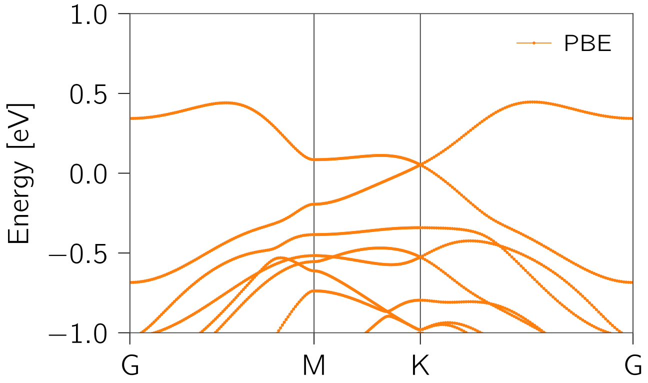


DFT band structure

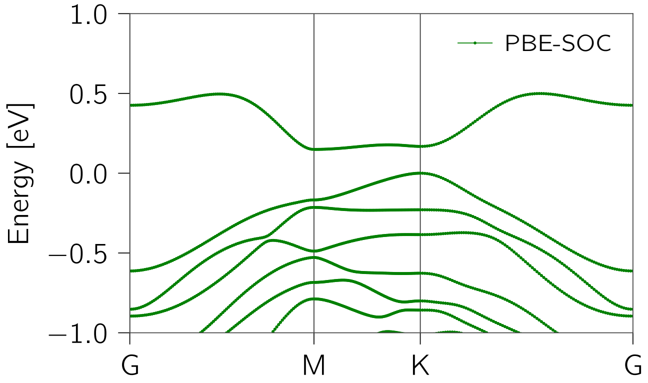


DFT band structure with spin-orbit coupling

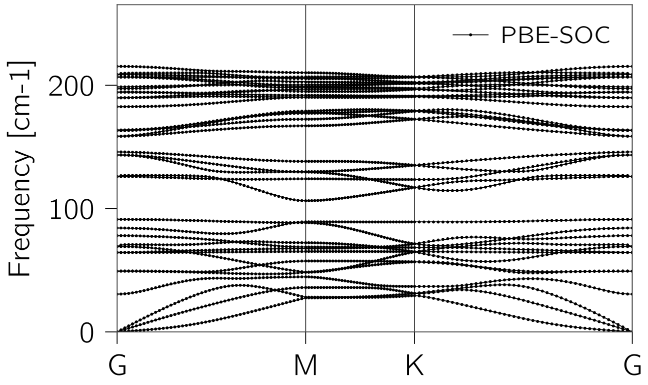


DFPT phonons dispersions

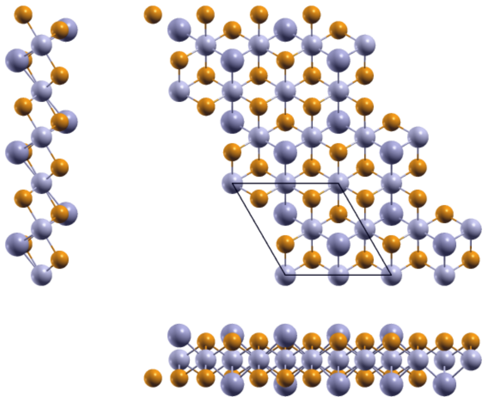

Orthographic projections

Se atoms are orange, Hg atoms are grey, Pt atoms are light grey.

Structural parameters: relaxed cell and atomic positions in cartesian coordinates

| | $x$ [Å] | $y$ [Å] | $z$ [Å] |
|---|---|---|---|
| $\boldsymbol{a_1}$ | 7.51386670 | 0.00000000 | 0.00000000 |
| $\boldsymbol{a_2}$ | −3.75693330 | 6.50719940 | 0.00000000 |
| $\boldsymbol{a_3}$ | 0.00000000 | 0.00000000 | 23.73722050 |
| Hg | 3.75693330 | 2.16906650 | 13.59575210 |
| Hg | 0.00000000 | 4.33813300 | 10.14146840 |
| Se | 1.85924220 | 5.41156700 | 13.15334040 |
| Se | 0.00000000 | 2.19126500 | 13.15334040 |
| Se | −1.85924220 | 5.41156700 | 13.15334040 |
| Se | 1.89769110 | 1.09563250 | 10.58388010 |
| Se | 3.75693330 | 4.31593450 | 10.58388010 |
| Se | 5.61617560 | 1.09563250 | 10.58388010 |
| Pt | −0.00000000 | −0.00000000 | 11.86861030 |
| Pt | 3.75693330 | 0.00000000 | 11.86861030 |
| Pt | 1.87846670 | 3.25359970 | 11.86861030 |
| Pt | −1.87846670 | 3.25359970 | 11.86861030 |

# $TaRhTe_4$

## Info and properties

**Formula (DB ID)** $TaRhTe_4$ (ICSD 656453)
**Spacegroup** P$m$ (6)
**DFT band gap [meV]** 65
**DFT inversion strength [meV]** 215

**No. atoms per unit cell** 12
**DF2-C09 Binding energy [meV/Å$^2$]** 26
**rVV10 Binding energy [meV/Å$^2$]** 31

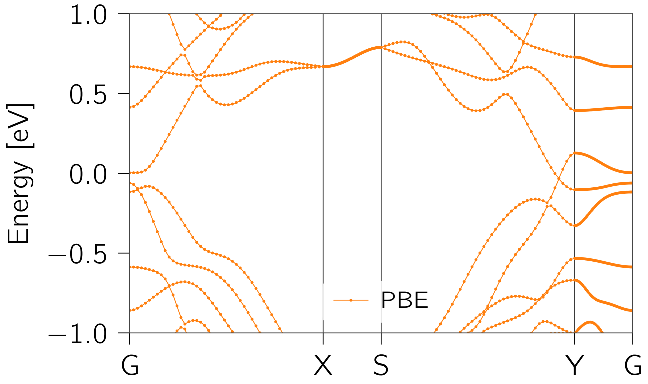


DFT band structure

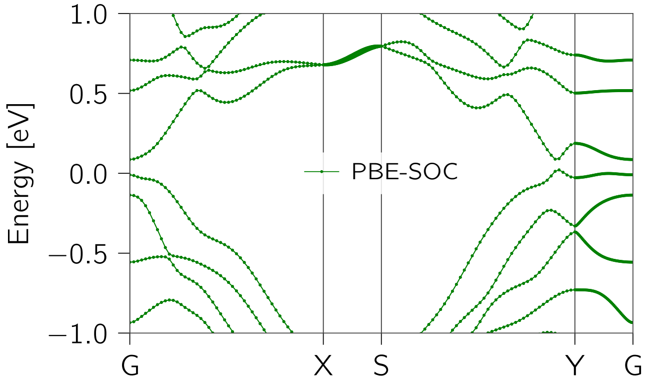


DFT band structure with spin-orbit coupling

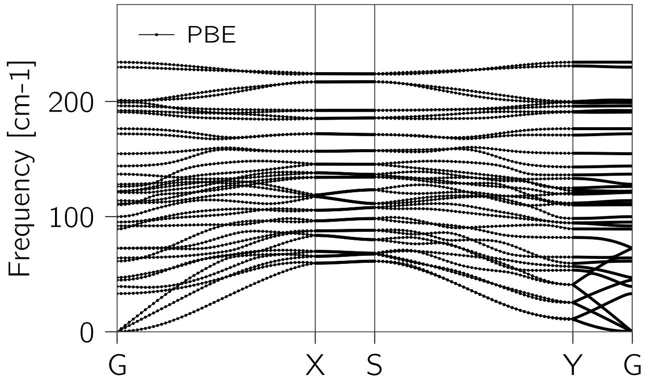


DFPT phonons dispersions

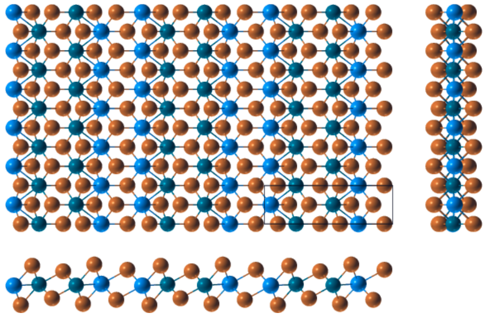

Orthographic projections
Te atoms are brown, Ta atoms are blue, Rh atoms are dark blue.

Structural parameters: relaxed cell and atomic positions in cartesian coordinates

| | $x$ [Å] | $y$ [Å] | $z$ [Å] |
|---|---|---|---|
| $\boldsymbol{a_1}$ | 3.79877069 | 0.00000000 | 0.00000000 |
| $\boldsymbol{a_2}$ | 0.00000000 | 12.66402983 | 0.00000000 |
| $\boldsymbol{a_3}$ | 0.00000000 | 0.00000000 | 38.02810594 |
| Ta | 0.00000000 | 3.39477922 | −0.08498765 |
| Ta | 1.89938535 | 12.02243408 | 0.08479467 |
| Te | 1.89938535 | 8.25812803 | 1.33340490 |
| Te | 1.89938535 | 1.92386339 | 1.48489936 |
| Te | 1.89938535 | 4.09202662 | −1.99954489 |
| Te | 0.00000000 | 7.15903228 | −1.33314874 |
| Te | 0.00000000 | 5.20620339 | 1.88625392 |
| Te | 0.00000000 | 0.82930790 | −1.48513286 |
| Te | 0.00000000 | 11.32542965 | 1.99943371 |
| Te | 1.89938535 | 10.21070866 | −1.88616138 |
| Rh | 0.00000000 | 9.53690694 | −0.04185466 |
| Rh | 1.89938535 | 5.88023215 | 0.04204363 |

# $WTe_2$

## Info and properties

**Formula (DB ID)** $WTe_2$ (COD 2310355)
**Spacegroup** $P2_1/m$ (11)
**DFT band gap [meV]** 9 (at 2 % strain)
**DFT inversion strength [meV]** 972

**No. atoms per unit cell** 6
**DF2-C09 Binding energy [meV/Å$^2$]** 30
**rVV10 Binding energy [meV/Å$^2$]** 27

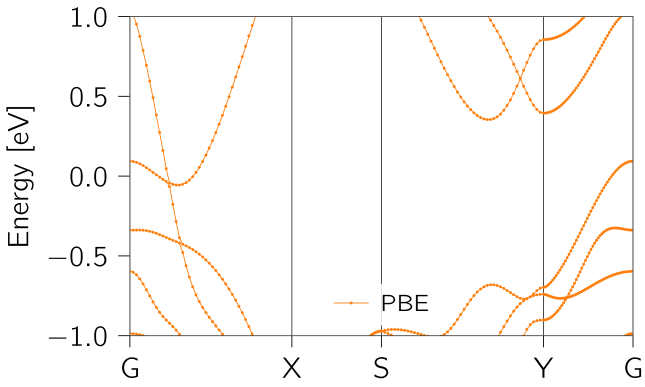


DFT band structure

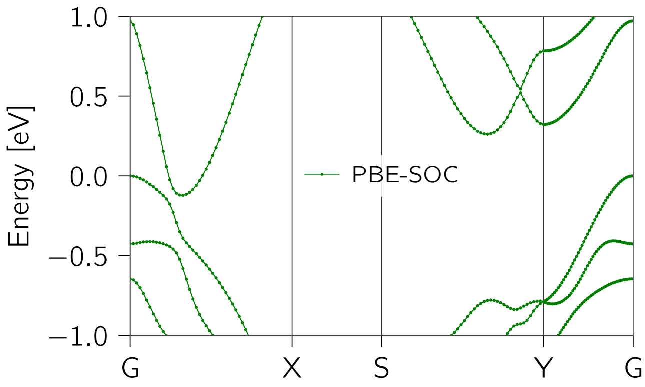


DFT band structure with spin-orbit coupling

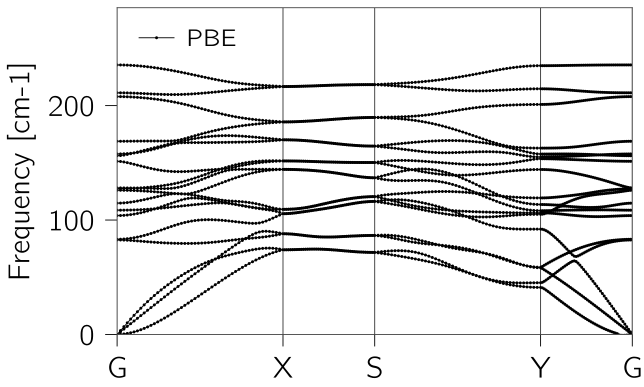


DFPT phonons dispersions

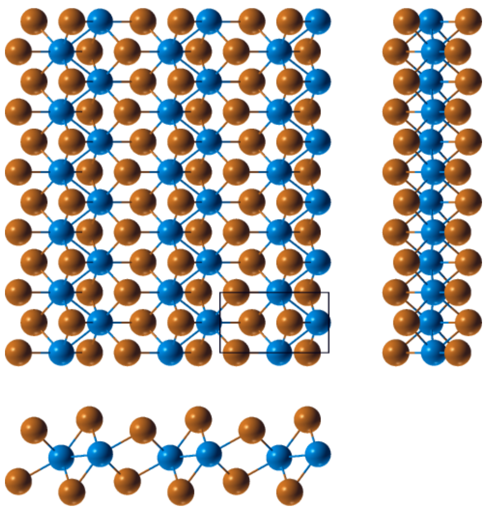

Orthographic projections

W atoms are blue, Te atoms are brown.

Structural parameters: relaxed cell and atomic positions in cartesian coordinates

| | $x$ [Å] | $y$ [Å] | $z$ [Å] |
|---|---|---|---|
| $\boldsymbol{a_1}$ | 3.49805086 | 0.00000000 | 0.00000000 |
| $\boldsymbol{a_2}$ | 0.00000000 | 6.32740661 | 0.00000000 |
| $\boldsymbol{a_3}$ | 0.00000000 | 0.00000000 | 24.22085657 |
| Te | 0.00000000 | 1.24934154 | 10.00235419 |
| Te | 1.74902543 | 4.47136176 | 10.62489260 |
| Te | 1.74902543 | 2.27111174 | 14.21720012 |
| Te | 0.00000000 | 5.37653650 | 13.59465094 |
| W | 0.00000000 | 2.88450804 | 12.21179413 |
| W | 1.74902543 | 0.63597840 | 12.00775719 |

# $In_2ZnS_4$

## Info and properties

**Formula (DB ID)** $In_2ZnS_4$ (ICSD 44637)

**Spacegroup** P3$m$1 (156)

**DFT band gap [meV]** 0

**DFT inversion strength [meV]** 191

**No. atoms per unit cell** 7

**DF2-C09 Binding energy [meV/Å$^2$]** 36

**rVV10 Binding energy [meV/Å$^2$]** 39

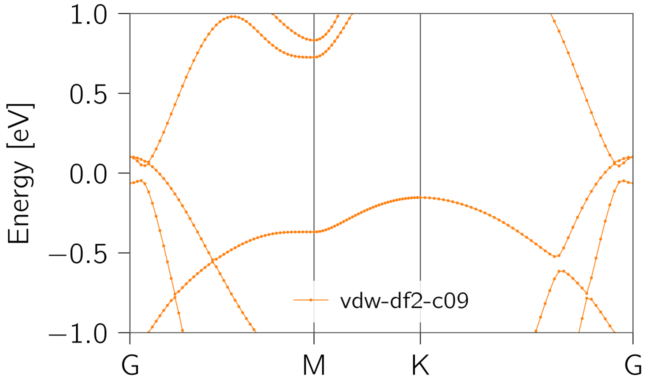


DFT band structure

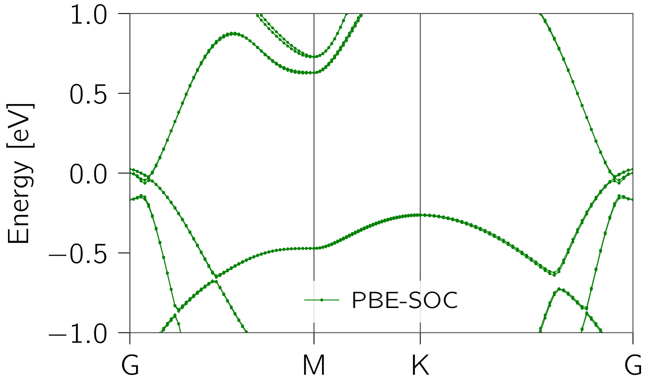


DFT band structure with spin-orbit coupling

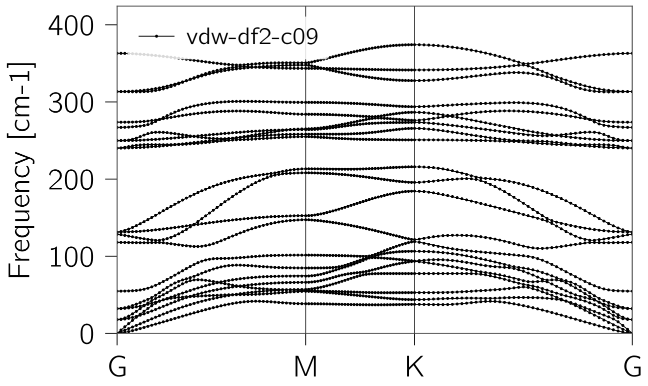


DFPT phonons dispersions

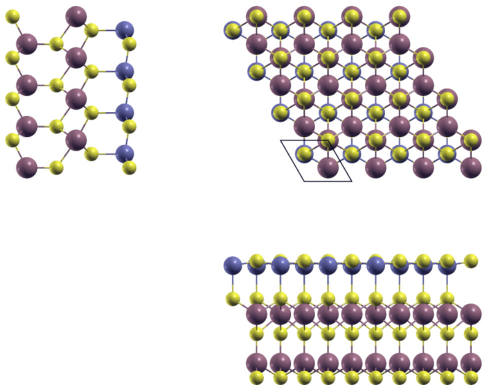

Orthographic projections

Zn atoms are blue, In atoms are purple, S atoms are yellow.

Structural parameters: relaxed cell and atomic positions in cartesian coordinates

| | $x$ [Å] | $y$ [Å] | $z$ [Å] |
|---|---|---|---|
| $\boldsymbol{a_1}$ | 3.86926032 | 0.00000000 | 0.00000000 |
| $\boldsymbol{a_2}$ | −1.93463016 | 3.35087773 | 0.00000000 |
| $\boldsymbol{a_3}$ | 0.00000000 | 0.00000000 | 29.47927669 |
| In | 1.93463016 | 1.11695924 | 18.38283886 |
| S | 1.93463016 | 1.11695924 | 15.97397963 |
| In | 1.93463016 | 3.35087773 | 14.37532168 |
| S | 1.93463016 | 3.35087773 | 19.54664707 |
| Zn | −0.00000000 | 2.23391849 | 10.42873407 |
| S | −0.00000000 | 2.23391849 | 13.13839630 |
| S | 1.93463016 | 1.11695924 | 10.05747957 |
